# Supplementary material for: A time-to-event three-outcome design for randomized phase II cancer trials
Source: arXiv:2503.15418 source file (2025-03-19)
Supplement: Supplementary file 1 [file appendix.tex]

# R function for determining minimum required sample size (#events) and boundaries with no IA
# hr0 - HR under H0
# hr1 - HR under H1
# note: hr1 must be less than hr0
#       alpha+eta must be <= 1
#       beta+pi must be <= 1
# r - randomization ratio (e.g. 1 for 1:1, 2 for 2:1)
# round.events - boolean. whether # events should be rounded up
tte3o.design<-function(hr0, hr1, alpha, beta, pi, eta, r=1, round.events=T)
\{
 theta0<-log(hr0)
 theta1<-log(hr1)
 z_pi<-qnorm(pi)
 z_alpha<-qnorm(alpha)
 z_beta<-qnorm(beta)
 z_eta<-qnorm(eta)
 bnd1<-(z_pi*theta0-z_alpha*theta1)/(z_pi-z_alpha) #lower boundary on log-scale
 bnd0<-(z_eta*theta1-z_beta*theta0)/(z_eta-z_beta) #upper boundary on log-scale
 d0<-((z_pi-z_alpha)/(theta0-theta1))^2 / (r/((1+r)^2))
 d1<-((z_eta-z_beta)/(theta0-theta1))^2 / (r/((1+r)^2))
 if (round.events)
     \{
      d0<-ceiling(d0)
      z_pi<-z_alpha+sqrt(d0*r)*(theta0-theta1)/(1+r)
      pi<-pnorm(z_pi)
      bnd1<-(z_pi*theta0-z_alpha*theta1)/(z_pi-z_alpha)
      d1<-ceiling(d1)
      z_beta<-z_eta-sqrt(d1*r)*(theta0-theta1)/(1+r)
      beta<-pnorm(z_beta)
      bnd0<-(z_eta*theta1-z_beta*theta0)/(z_eta-z_beta)
     \}
 if (d0>d1)
     \{
      z_beta<-z_eta-sqrt(d0*r)*(theta0-theta1)/(1+r)
      beta<-pnorm(z_beta)
      bnd0<-(z_eta*theta1-z_beta*theta0)/(z_eta-z_beta)
     \}
 else if (d1>d0)
     \{
      z_pi<-z_alpha+sqrt(d1*r)*(theta0-theta1)/(1+r)
      pi<-pnorm(z_pi)
      bnd1<-(z_pi*theta0-z_alpha*theta1)/(z_pi-z_alpha)
     \}
 c(hr0=hr0, hr1=hr1, n.events=d0, boundary.lower=exp(bnd1), boundary.upper=exp(bnd0),
     alpha.actual=alpha, beta.actual=beta, pi.actual=pi, eta.actual=eta, rand.ratio=r)
\}
